# Supplementary material for: Performance Analysis and Modeling of Video Transcoding Using Heterogeneous Cloud Services
Source: arXiv:1809.06529 source file (2018-09-18)
Supplement: Supplementary file 1 [file appendix.tex]

\section{}\label{FirstAppendix}
The following figures show the execution time of codec transcoding for all video in the benchmark on different VM types. We can observe that, in general, \texttt{GPU} VM provides a better execution time in compare with other VM types. \texttt{General} VM provides the lowest performance as it includes less powerful processing units.
\begin{figure*}[htbp]
    \centering
    \begin{subfigure}[b]{0.22\textwidth}
      \centering
      \includegraphics[width=\linewidth]{fig/all_codec/beamextract_final_revb}
      \caption{}
    \end{subfigure}
    \begin{subfigure}[b]{0.22\textwidth}
      \centering
      \includegraphics[width=\linewidth]{fig/all_codec/big_buck_bunny_480p_30mb}
      \caption{}
    \end{subfigure}
    \begin{subfigure}[b]{0.22\textwidth}
      \centering
      \includegraphics[width=\linewidth]{fig/all_codec/big_buck_bunny_720p_h264_01}
      \caption{}
    \end{subfigure}
    \begin{subfigure}[b]{0.22\textwidth}
      \centering
      \includegraphics[width=\linewidth]{fig/all_codec/big_buck_bunny_720p_h264_02}
      \caption{}
    \end{subfigure}
    \begin{subfigure}[b]{0.22\textwidth}
      \centering
      \includegraphics[width=\textwidth]{fig/all_codec/big_buck_bunny_720p_h264_03}
      \caption{}
    \end{subfigure}
    \begin{subfigure}[b]{0.22\textwidth}
      \centering
      \includegraphics[width=\textwidth]{fig/all_codec/big_buck_bunny_720p_h264_04}
      \caption{}
    \end{subfigure}
    \begin{subfigure}[b]{0.22\textwidth}
      \centering
      \includegraphics[width=\textwidth]{fig/all_codec/big_buck_bunny_720p_h264_05}
      \caption{}
    \end{subfigure}
    \begin{subfigure}[b]{0.22\textwidth}
      \centering
      \includegraphics[width=\textwidth]{fig/all_codec/big_buck_bunny_720p_stereo01}
      \caption{}
    \end{subfigure}
    \begin{subfigure}[b]{0.22\textwidth}
      \centering
      \includegraphics[width=\textwidth]{fig/all_codec/big_buck_bunny_720p_stereo02}
      \caption{}
    \end{subfigure}
    \begin{subfigure}[b]{0.22\textwidth}
      \centering
      \includegraphics[width=\textwidth]{fig/all_codec/big_buck_bunny_720p_stereo03}
      \caption{}
    \end{subfigure}
    \begin{subfigure}[b]{0.22\textwidth}
      \centering
      \includegraphics[width=\textwidth]{fig/all_codec/fantastic01}
      \caption{}
    \end{subfigure}
    \begin{subfigure}[b]{0.22\textwidth}
      \centering
      \includegraphics[width=\textwidth]{fig/all_codec/fantastic02}
      \caption{}
    \end{subfigure}
    \begin{subfigure}[b]{0.22\textwidth}
      \centering
      \includegraphics[width=\textwidth]{fig/all_codec/fantastic03}
      \caption{}
    \end{subfigure}
    \begin{subfigure}[b]{0.22\textwidth}
      \centering
      \includegraphics[width=\textwidth]{fig/all_codec/orion_sm}
      \caption{}
    \end{subfigure}
    \begin{subfigure}[b]{0.22\textwidth}
      \centering
      \includegraphics[width=\textwidth]{fig/all_codec/serenity_trailer01}
      \caption{}
    \end{subfigure}
    \begin{subfigure}[b]{0.22\textwidth}
      \centering
      \includegraphics[width=\textwidth]{fig/all_codec/serenity_trailer02}
      \caption{}
    \end{subfigure}
    \begin{subfigure}[b]{0.22\textwidth}
      \centering
      \includegraphics[width=\textwidth]{fig/all_codec/serenity_trailer03}
      \caption{}
    \end{subfigure}
    \begin{subfigure}[b]{0.22\textwidth}
      \centering
      \includegraphics[width=\textwidth]{fig/all_codec/serenity_trailer04}
      \caption{}
    \end{subfigure}
    \begin{subfigure}[b]{0.22\textwidth}
      \centering
      \includegraphics[width=\textwidth]{fig/all_codec/simpsons_trailer01}
      \caption{}
    \end{subfigure}
    \begin{subfigure}[b]{0.22\textwidth}
      \centering
      \includegraphics[width=\textwidth]{fig/all_codec/simpsons_trailer02}
      \caption{}
    \end{subfigure}
    \begin{subfigure}[b]{0.22\textwidth}
      \centering
      \includegraphics[width=\textwidth]{fig/all_codec/simpsons_trailer03}
      \caption{}
    \end{subfigure}
    \begin{subfigure}[b]{0.22\textwidth}
      \centering
      \includegraphics[width=\textwidth]{fig/all_codec/simpsons_trailer04}
      \caption{}
    \end{subfigure}
    \begin{subfigure}[b]{0.22\textwidth}
      \centering
      \includegraphics[width=\textwidth]{fig/all_codec/simpsons_trailer05}
      \caption{}
    \end{subfigure}
    \begin{subfigure}[b]{0.22\textwidth}
      \centering
      \includegraphics[width=\textwidth]{fig/all_codec/simpsons_trailer06}
      \caption{}
    \end{subfigure}

    \label{fig:vm_type}
\end{figure*}
